# Supplementary material for: Khovanov homology and the Involutive Heegaard Floer homology of branched double covers
Source: arXiv:2305.07172 source file (2023-05-11)
Supplement: Supplementary file 1 [file AZ-bimod.tex]

\documentclass[crop]{standalone}
\input{commands}

\begin{document}

\begin{tikzpicture}
% variables
\def\w{6} % width variable
\def\h{8} % height, general size dimension
\def\gap{.3} % offset space of labels
% lines
\draw (0,0) -- (0,\h);
\draw (\h,0) -- (\h,\h);
\draw (0,\h) -- (\h, \h);
% handles
\node[label={$\iota_1$}] (i1L) at (1,\h) {$\newmoon$};
\node[label={$\iota_0$}] (i0L) at (3,\h) {$\fullmoon$};
\node[label={$\iota_1$}] (i1R) at (5,\h) {$\newmoon$};
\node[label={$\iota_0$}] (i0R) at (7,\h) {$\fullmoon$};
% boundary labels
\foreach \k in {1,2,3,4} {
    \node at (0-\gap, -1+2*\k) {$\k$};
    \node at (\h+\gap, \h+1-2*\k) {$\k$};
}
% alpha arcs
\foreach \k in {1,2,3,4} {
    \draw[red] (0, -1+2*\k) -- (\h+1-2*\k,\h);
}
% beta arcs
\foreach \k in {1,2,3,4} {
    \draw[blue] (\h+1-2*\k,\h) -- (\h, \h+1-2*\k);
}
% more labels
\node[label={$\ro{3,4}$}] at (2,7) {};
\node[label={$\ro{2,3}$}] at (4,7) {};
\node[label={$\ro{1,2}$}] at (6,7) {};
\node[label={$\ro{2,4}$}] at (3,6) {};
\node[label={$\ro{1,3}$}] at (5,6) {};
\node[label={$\ro{1,4}$}] at (4,5) {};
\end{tikzpicture}

\end{document}
