# Supplementary material for: Khovanov homology and the Involutive Heegaard Floer homology of branched double covers
Source: arXiv:2305.07172 source file (2023-05-11)
Supplement: Supplementary file 3 [file dOmega.tex]

\documentclass[crop]{standalone}
\input{commands}
\usepackage{scalerel}

\begin{document}

\begin{tikzpicture}[xscale=1.5]
% nodes
\node (partial) at (0,1) {$\delta^{\mathrm{Id}}$};
\node (Omega) at (0,0) {$\Omega$};
\node (delta) at (0,-1) {$\deltaAZAZ$};
\node (mu) at (-1,-1.5) {$\mu$};
\node (splitter) at (.7,1.5) {$\Delta$};
\node (in-alg) at (1.5,2) {};
\node (out-alg) at (-1.5,-2) {};
\node (input) at (0, 2) {};
\node (output) at (0,-2) {};
% arcs
\draw[-stealth, dashed] (input) -- (partial);
\draw[-stealth, dashed] (partial) -- (Omega);
\draw[-stealth, dashed] (Omega) -- (delta);
\draw[-stealth, dashed] (delta) -- (output);
\draw[double, -stealth] (in-alg) -- (splitter);
\draw[-stealth] (mu) -- (out-alg);
\draw[-stealth] (splitter) -- (partial);
\draw[-stealth] (splitter) -- (Omega);
\draw[-stealth] (splitter) -- (delta);
%
% \draw[->] (partial) to [out=220, in=90] (mu);
\draw[-stealth] (partial) -- (mu);
\draw[-stealth] (Omega) -- (mu);
\draw[-stealth] (delta) -- (mu);
\end{tikzpicture}
%%%%%%%%%%%%%%%%%%%%%%%%%%%%%%%%%%%%%%%%%
\begin{tikzpicture}[xscale=1.5]
% nodes
\node (Omega) at (0,0) {$\Omega$};
\node (Dbar) at (.7,1.5) {$\ovl D$};
\node (in-alg) at (1.5,2) {};
\node (out-alg) at (-1,-2) {};
\node (input) at (0, 2) {};
\node (output) at (0,-2) {};
% arcs
\draw[-stealth, dashed] (input) -- (Omega);
\draw[-stealth, dashed] (Omega) -- (output);
\draw[double,stealth-] (Dbar) -- (in-alg);
\draw[-stealth] (Dbar) -- (Omega);
\draw[-stealth] (Omega) -- (out-alg);
\end{tikzpicture}

\end{document}
