# Supplementary material for: Khovanov homology and the Involutive Heegaard Floer homology of branched double covers
Source: arXiv:2305.07172 source file (2023-05-11)
Supplement: Supplementary file 6 [file dOmega_3.tex]

\documentclass[crop]{standalone}
\input{commands}

\begin{document}

\begin{tikzpicture}
% nodes
\node (partial) at (0,1) {$\delta^1_2$};
\node (Omega) at (0,0) {$\Omega^1_2$};
%\node (delta) at (0,-1) {$\delta$};
\node (mu) at (-1,-1.5) {$\mu$};
\node (splitter) at (1,1.5) {$\Delta$};
\node (in-alg) at (1.5,2.5) {};
\node (out-alg) at (-1.5,-2) {};
\node (input) at (0, 2.5) {};
\node (output) at (0,-2) {};
% arcs
\draw[-stealth, dashed] (input) edge (partial);
\draw[-stealth, dashed] (partial) edge (Omega);
%\draw (Omega) -- (delta);
\draw[stealth-, dashed] (output) edge (Omega);
\draw[double,stealth-] (splitter) -- (in-alg);
\draw[-stealth] (mu) edge (out-alg);
\draw[-stealth] (splitter) edge (partial);
\draw[-stealth] (splitter) edge (Omega);
%\draw (splitter) -- (delta);
%
\draw[stealth-] (mu) edge (partial);
\draw[stealth-] (mu) edge (Omega);
%\draw (mu) -- (delta);
\end{tikzpicture}

%%%%%%%%%%%%%%%%%%%%%%%%%%%%%%%%%%%%%%%%%%%%%%%%%%%%%

\begin{tikzpicture}
% nodes
%\node (partial) at (0,1) {$\partial$};
\node (Omega) at (0,0) {$\Omega^1_2$};
\node (delta) at (0,-1) {$\delta^1_2$};
\node (mu) at (-1,-1.5) {$\mu$};
\node (splitter) at (1,1.5) {$\Delta$};
\node (in-alg) at (1.5,2.5) {};
\node (out-alg) at (-1.5,-2) {};
\node (input) at (0, 2.5) {};
\node (output) at (0,-2) {};
% arcs
\draw[-stealth, dashed] (input) edge (Omega);
%\draw (partial) -- (Omega);
\draw[-stealth, dashed] (Omega) edge (delta);
\draw[stealth-, dashed] (output) edge (delta);
\draw[double, stealth-] (splitter) -- (in-alg);
\draw[-stealth] (mu) edge (out-alg);
%
%\draw (splitter) -- (partial);
\draw[-stealth] (splitter) edge (Omega);
\draw[-stealth] (splitter) edge (delta);
%
%\draw (mu) -- (partial);
\draw[stealth-] (mu) edge (Omega);
\draw[stealth-] (mu) edge (delta);
\end{tikzpicture}

%%%%%%%%%%%%%%%%%%%%%%%%%%%%%%%%%%%%%%%%%%%%%%%%%%%%%%%

\begin{tikzpicture}
% nodes
%\node (partial) at (0,1) {$\partial$};
\node (Omega) at (0,0) {$\Omega_2^1$};
%\node (delta) at (0,-1) {$\delta$};
%\node (mu) at (-1,-1.5) {$\mu$};
\node (splitter) at (1,1.5) {$\mu_2$};
\node (in-alg) at (1.5,2.5) {};
\node (out-alg) at (-1.5,-2) {};
\node (input) at (0, 2.5) {};
\node (output) at (0,-2) {};
% arcs
\draw[-stealth] (splitter) edge (Omega);
\draw[double,-stealth] (in-alg) -- (splitter);
\draw[-stealth, dashed] (input) edge (Omega);
\draw[stealth-, dashed] (output) edge (Omega);
\draw[stealth-] (out-alg) edge (Omega);

\end{tikzpicture}

%%%%%%%%%%%%%%%%%%%%%%%%%%%%%%%%%%%%%%%%%%%%%%%%%%%%%

\begin{tikzpicture}
% nodes
%\node (partial) at (0,1) {$\partial$};
\node (Omega) at (0,0) {$\Omega^1_3$};
\node (delta) at (0,-1) {$\delta^1_1$};
\node (mu) at (-1,-1.5) {$\mu$};
%\node (splitter) at (1,1.5) {$\Delta$};
\node (in-alg) at (1.5,2.5) {};
\node (out-alg) at (-1.5,-2) {};
\node (input) at (0, 2.5) {};
\node (output) at (0,-2) {};
% arcs
\draw[-stealth, dashed] (input) edge (Omega);
%\draw (partial) -- (Omega);
\draw[-stealth, dashed] (Omega) edge (delta);
\draw[stealth-, dashed] (output) edge (delta);
\draw[double, stealth-] (Omega) -- (in-alg);
\draw[-stealth] (mu) edge (out-alg);
%
%\draw (splitter) -- (partial);
%\draw (splitter) -- (Omega);
%\draw (splitter) -- (delta);
%
%\draw (mu) -- (partial);
\draw[stealth-] (mu) edge (Omega);
\draw[stealth-] (mu) edge (delta);
\end{tikzpicture}

\end{document}
