# Supplementary material for: Khovanov homology and the Involutive Heegaard Floer homology of branched double covers
Source: arXiv:2305.07172 source file (2023-05-11)
Supplement: Supplementary file 7 [file dOmega_4.tex]

\documentclass[crop, varwidth]{standalone}
\input{commands}

\begin{document}

\begin{tikzpicture}
% nodes
\node (partial) at (0,1) {$\partial^1_2$};
\node (Omega) at (0,0) {$\Omega^1_3$};
%\node (delta) at (0,-1) {$\delta$};
\node (mu) at (-1,-1.5) {$\mu$};
\node (splitter) at (1,1.5) {$\Delta$};
\node (in-alg) at (2,2) {};
\node (out-alg) at (-1.5,-2) {};
\node (input) at (0, 2) {};
\node (output) at (0,-2) {};
% arcs
\draw[-stealth, dashed] (input) -- (partial);
\draw[-stealth, dashed] (partial) -- (Omega);
%\draw (Omega) -- (delta);
\draw[-stealth, dashed] (Omega) -- (output);
\draw[double, -stealth] (in-alg) -- (splitter);
\draw[-stealth] (mu) -- (out-alg);
\draw[-stealth] (splitter) -- (partial);
\draw[double, -stealth] (splitter) -- (Omega);
%\draw (splitter) -- (delta);
%
\draw[-stealth] (partial) -- (mu);
\draw[-stealth] (Omega) -- (mu);
%\draw (mu) -- (delta);
\end{tikzpicture}
%
%%%%%%%%%%%%%%%%%%%%%%%%%%%%%%%%%%%%%%%%%%%%%%%%%%%%%%%%%%%%
%
\begin{tikzpicture}
% nodes
%\node (partial) at (0,1) {$\partial$};
\node (Omega) at (0,0) {$\Omega^1_3$};
\node (delta) at (0,-1) {$\delta^1_2$};
\node (mu) at (-1,-1.5) {$\mu$};
\node (splitter) at (1,1.5) {$\Delta$};
\node (in-alg) at (2,2) {};
\node (out-alg) at (-1.5,-2) {};
\node (input) at (0, 2) {};
\node (output) at (0,-2) {};
% arcs
\draw[-stealth,dashed] (input) -- (Omega);
%\draw (partial) -- (Omega);
\draw[-stealth,dashed] (Omega) -- (delta);
\draw[-stealth,dashed] (delta) -- (output);
\draw[double, -stealth] (in-alg) -- (splitter);
\draw[-stealth] (mu) -- (out-alg);
%
%\draw (splitter) -- (partial);
\draw[double, -stealth] (splitter) -- (Omega);
\draw[-stealth] (splitter) -- (delta);
%
%\draw (mu) -- (partial);
\draw[-stealth] (Omega) -- (mu);
\draw[-stealth] (delta) -- (mu);
\end{tikzpicture}
%
%%%%%%%%%%%%%%%%%%%%%%%%%%%%%%%%%%%%%%%%%%%%%%%%%%%%%%%%%%%%
%
\begin{tikzpicture}
% nodes
%\node (partial) at (0,1) {$\partial$};
\node (Omega) at (0,0) {$\Omega^1_3$};
%\node (delta) at (0,-1) {$\delta$};
\node (mu) at (.7,1.5) {$\mu$};
% \node (splitter) at (1,1.5) {$\Delta$};
\node (in-alg1) at (1.5,2) {};
\node (in-alg2) at (2,2) {};
\node (out-alg) at (-1.5,-2) {};
\node (input) at (0, 2) {};
\node (output) at (0,-2) {};
% arcs
\draw[-stealth, dashed] (input) -- (Omega);
%\draw (partial) -- (Omega);
%\draw (Omega) -- (delta);
\draw[-stealth, dashed] (Omega) -- (output);
\draw[double, -stealth] (in-alg1) -- (mu);
\draw[-stealth] (mu) -- (Omega);
\draw[-stealth] (in-alg2) -- (Omega);
\draw[-stealth] (Omega) -- (out-alg);
%
%\draw (splitter) -- (partial);
%\draw (splitter) -- (Omega);
%\draw (splitter) -- (delta);
%
%\draw (mu) -- (partial);
%\draw (mu) -- (Omega);
%\draw (mu) -- (delta);
\end{tikzpicture}

%%%%%%%%%%%%%%%%%%%%%%%%%%%%%%%%%%%%%%%%%%%%%%%%%%%%%%%%%%%%

\begin{tikzpicture}
% nodes
%\node (partial) at (0,1) {$\partial$};
\node (Omega) at (0,0) {$\Omega^1_3$};
%\node (delta) at (0,-1) {$\delta$};
\node (mu) at (1,1) {$\mu$};
% \node (splitter) at (1,1.5) {$\Delta$};
\node (in-alg1) at (1,2) {};
\node (in-alg2) at (2,2) {};
\node (out-alg) at (-1.5,-2) {};
\node (input) at (0, 2) {};
\node (output) at (0,-2) {};
% arcs
\draw[-stealth, dashed] (input) -- (Omega);
%\draw (partial) -- (Omega);
%\draw (Omega) -- (delta);
\draw[-stealth, dashed] (Omega) -- (output);
\draw[double, -stealth] (in-alg2) -- (mu);
\draw[-stealth] (mu) -- (Omega);
\draw[-stealth] (in-alg1) -- (Omega);
\draw[-stealth] (Omega) -- (out-alg);
%
%\draw (splitter) -- (partial);
%\draw (splitter) -- (Omega);
%\draw (splitter) -- (delta);
%
%\draw (mu) -- (partial);
%\draw (mu) -- (Omega);
%\draw (mu) -- (delta);
\end{tikzpicture}
%
%%%%%%%%%%%%%%%%%%%%%%%%%%%%%%%%%%%%%%%%%%%%%%%%%%%%%%%%%%%%
%
\begin{tikzpicture}
% nodes
%\node (partial) at (0,1) {$\partial$};
\node (Omega) at (0,0) {$\Omega^1_4$};
\node (delta) at (0,-1) {$\delta^1_1$};
\node (mu) at (-1,-1.5) {$\mu$};
%\node (splitter) at (1,1.5) {$\Delta$};
\node (in-alg) at (1.5,2) {};
\node (out-alg) at (-1.5,-2) {};
\node (input) at (0, 2) {};
\node (output) at (0,-2) {};
% arcs
\draw[-stealth, dashed] (input) -- (Omega);
%\draw (partial) -- (Omega);
\draw[-stealth, dashed] (Omega) -- (delta);
\draw[-stealth, dashed] (delta) -- (output);
\draw[double, -stealth] (in-alg) -- node[midway,above] {3} ++ (Omega);
\draw[-stealth] (mu) -- (out-alg);
%
%\draw (splitter) -- (partial);
%\draw (splitter) -- (Omega);
%\draw (splitter) -- (delta);
%
%\draw (mu) -- (partial);
\draw[-stealth] (Omega) -- (mu);
\draw[-stealth] (delta) -- (mu);
\end{tikzpicture}

%%%%%%%%%%%%%%%%%%%%%%%%%%%%%%%%%%%%%%%%%%%%%%%%%%%%%%%%%%%%

\end{document}
